# Supplementary material for: Beyond mAP: Towards better evaluation of instance segmentation
Source: arXiv:2207.01614 source file (2023-03-20)
Supplement: Supplementary file 1 [file X_supplementary.tex]

\appendix

% --- PDF will be split by an editor (e.g. macOS preview), so need to restart from page 1
\setcounter{page}{1}

% --- repeat the title (AT: haven't found a more elegant way to do this...)
\twocolumn[
\centering
\Large
\textbf{Beyond mAP: Towards better evaluation of instance segmentation} \\
\vspace{0.5em}Supplementary Material \\
\vspace{1.0em}
] %< twocolumn
\appendix

% \begin{figure}
%     \centering
%     \includegraphics[width=\linewidth]{images/pseudoorientation.png}
%     \caption{ \textbf{Demonstration of the effectiveness of Pseudo-Orientation Flow:} Fig. (a) shows the input image and Fig. (b) shows the predicted POF. The remaining figures all predictions with greater than 0.5 confidence after MatrixNMS for various configurations. Fig. (a) shows the results of the base SOLOv2 model, Fig. (b) shows the results with the addition of the SS and CDF branches, Fig. (c) shows the results with only the POF branch, and Fig. (d) shows the results using all of the SS, CDF, and POF branches.}
%     \label{fig:pof}
% \end{figure}

\section{Behavior of PR curves in SOTA}
We make an unusual observation that state-of-the-art instance segmentation frameworks improve mAP, but also worsen the amount of \textit{hedged predictions}.
% To quantify, we analyze the PR curves of different frameworks \ie FastNMS, DETR, SOLOv2, QueryInst, and Mask NMS.
% This is shown in Fig.\ref{todo}.
% Note that modern segmentation frameworks suffer from hedging, and the last curve shows a huge FP to TP ratio in the high recall range.
Fig.\ref{fig:ap-ind} shows a side-by-side comparison between SOLOv2 with Matrix NMS and Mask NMS on individual images from the COCO validation dataset.
We observe that at an individual image level, AP is unable to detect or penalize hedging by construction.
This is detected using DC, NE, and LRP, and can be mitigated by our proposed Semantic Sorting and Semantic NMS modules.

\section{More Qualitative results in COCO validation dataset}
In this section, we compare segmentation quality in SOLOv2 and our method where we augment SOLOv2 with a shallow semantic segmentation module, which allows us to perform Semantic Sorting and Semantic NMS.
Results are shown in Fig.\ref{fig:solovours1}, \ref{fig:solovours2}, \ref{fig:solovours3}.
We prevent both spatial and category hedging on all images, leading to better qualitative and interpretable segmentation outputs.
In particular, we observe that our method outputs accurate counts of objects in the scene, which may be useful for applications like tracking and crowd counting.

%%%%%%%%%%%%%%%%%%%%%%%%%%%%%%%%%%%%%%%%
% this is where figures begin
%%%%%%%%%%%%%%%%%%%%%%%%%%%%%%%%%%%%%%%%

\begin{figure*}
    \centering
    \includegraphics[width=0.86\linewidth]{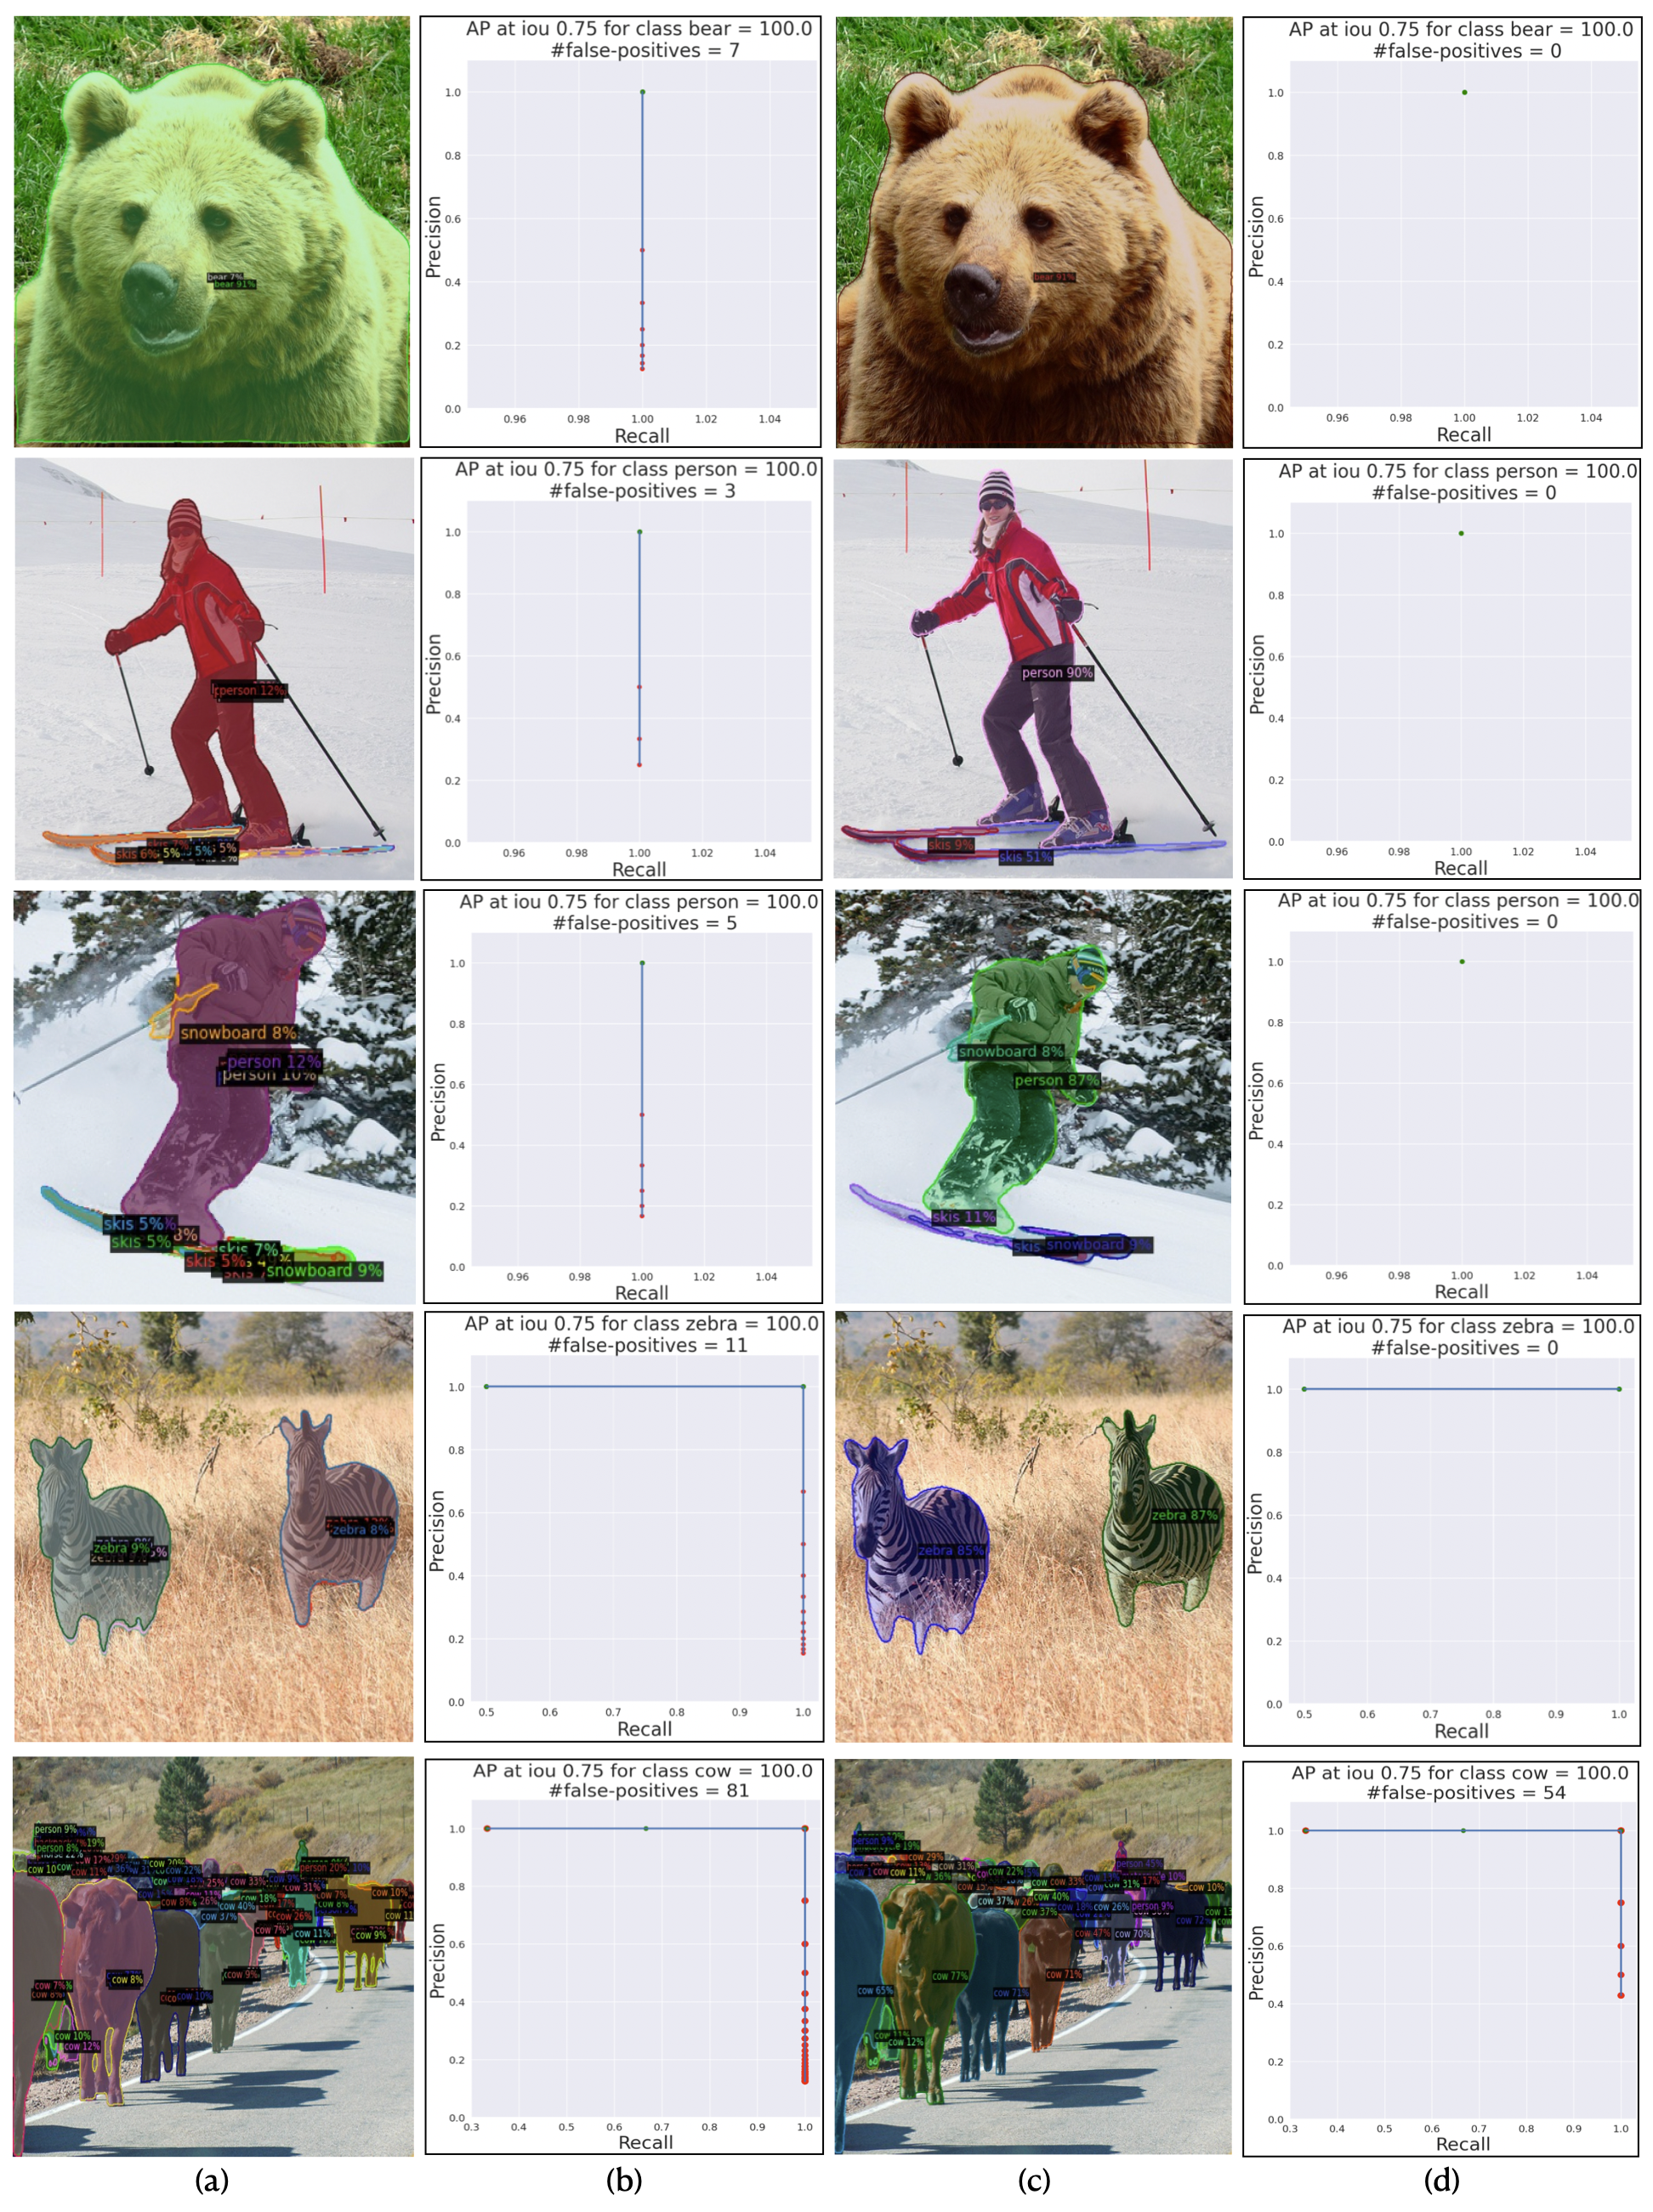}
    \caption{\textbf{AP and hedging}: (a) shows the
    prediction of SOLOv2 model with Matrix NMS, (b) shows the corresponding P/R
    curve. (c) shows the prediction with the same network but with Mask NMS, (d) shows
    the corresponding P/R curve. Note that despite having hedging (overcounting)
    in the first case, the AP scores are the same for both cases. However, they exhibit
    drastically different qualitative behavior, showing that AP is not an adequate metric
    for evaluating the hedging problem.}
    \label{fig:ap-ind}
\end{figure*}

\begin{figure*}
    \centering
    \includegraphics[width=0.95\linewidth]{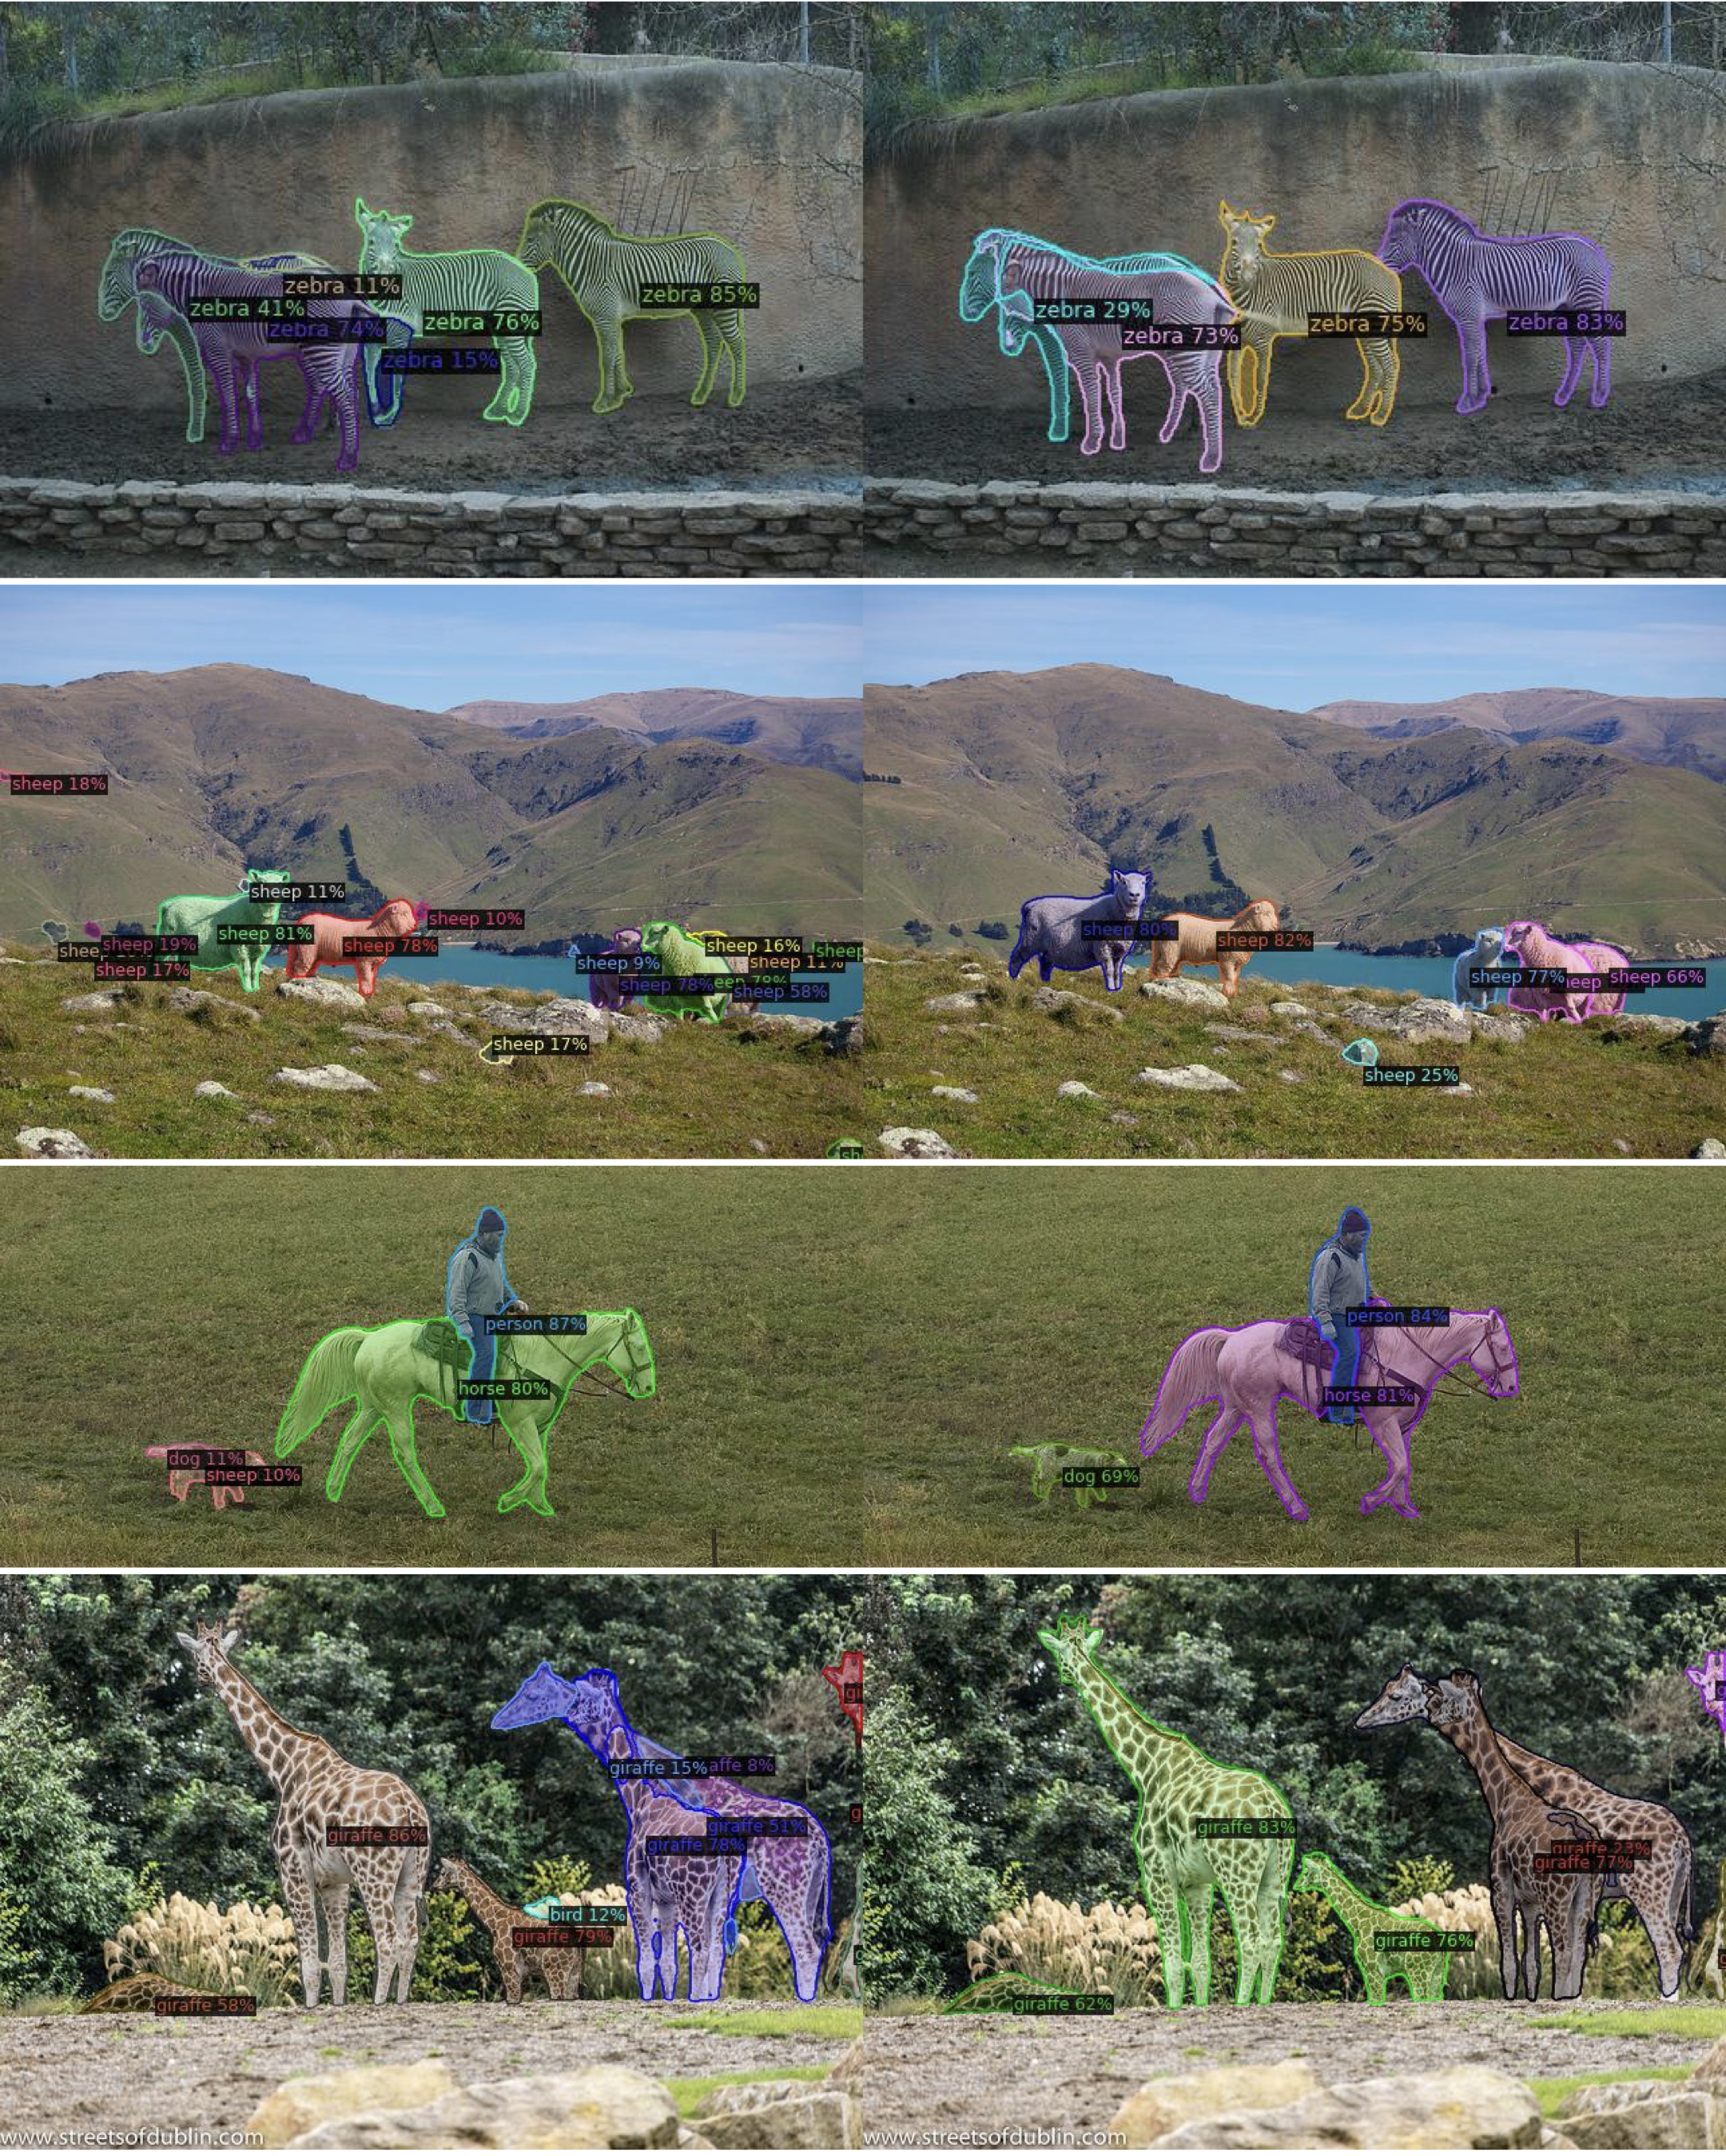}
    \caption{\textbf{Qualitative comparison on COCO-val-2017 dataset}: Images on left are predictions made by SOLOv2, images on right are predictions by our model with Semantic Sorting and Semantic NMS.}
    \label{fig:solovours1}
\end{figure*}
\begin{figure*}
    \centering
    \includegraphics[width=\linewidth]{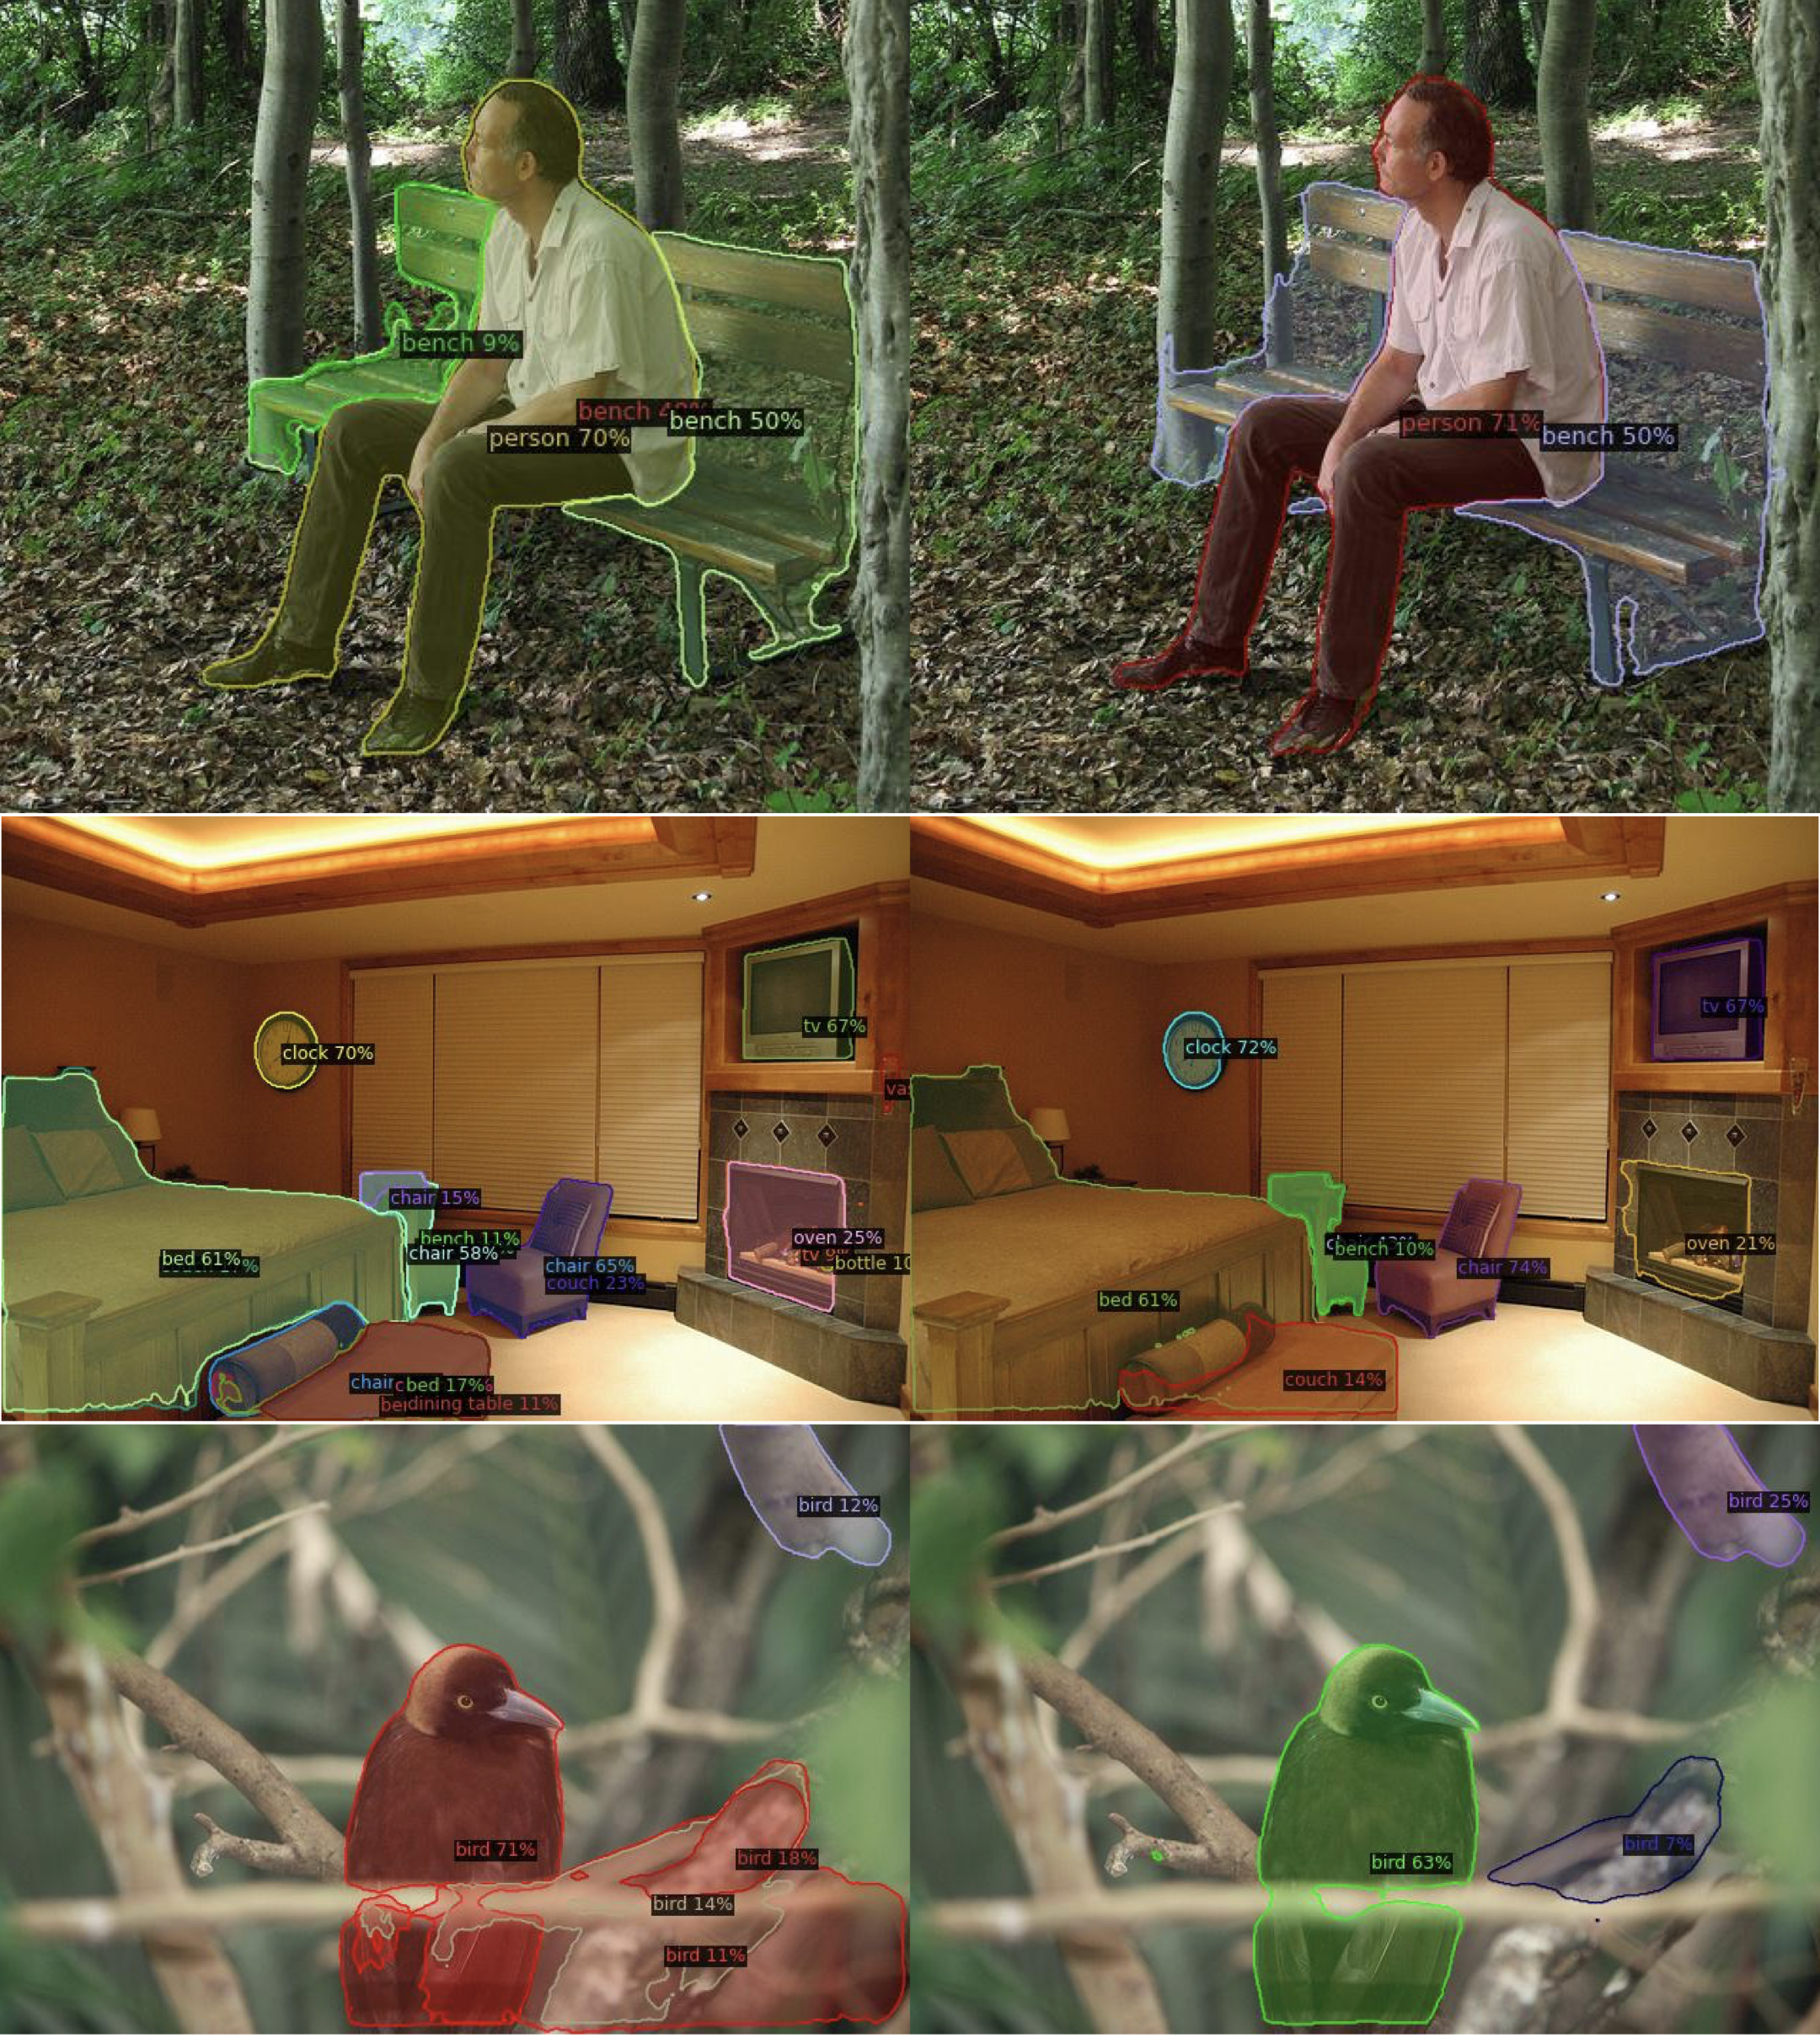}
    \caption{\textbf{Qualitative comparison on COCO-val-2017 dataset}: Images on left are predictions made by SOLOv2, images on right are predictions by our model with Semantic Sorting and Semantic NMS.}
    \label{fig:solovours2}
\end{figure*}
\begin{figure*}
    \centering
    \includegraphics[width=0.9\linewidth]{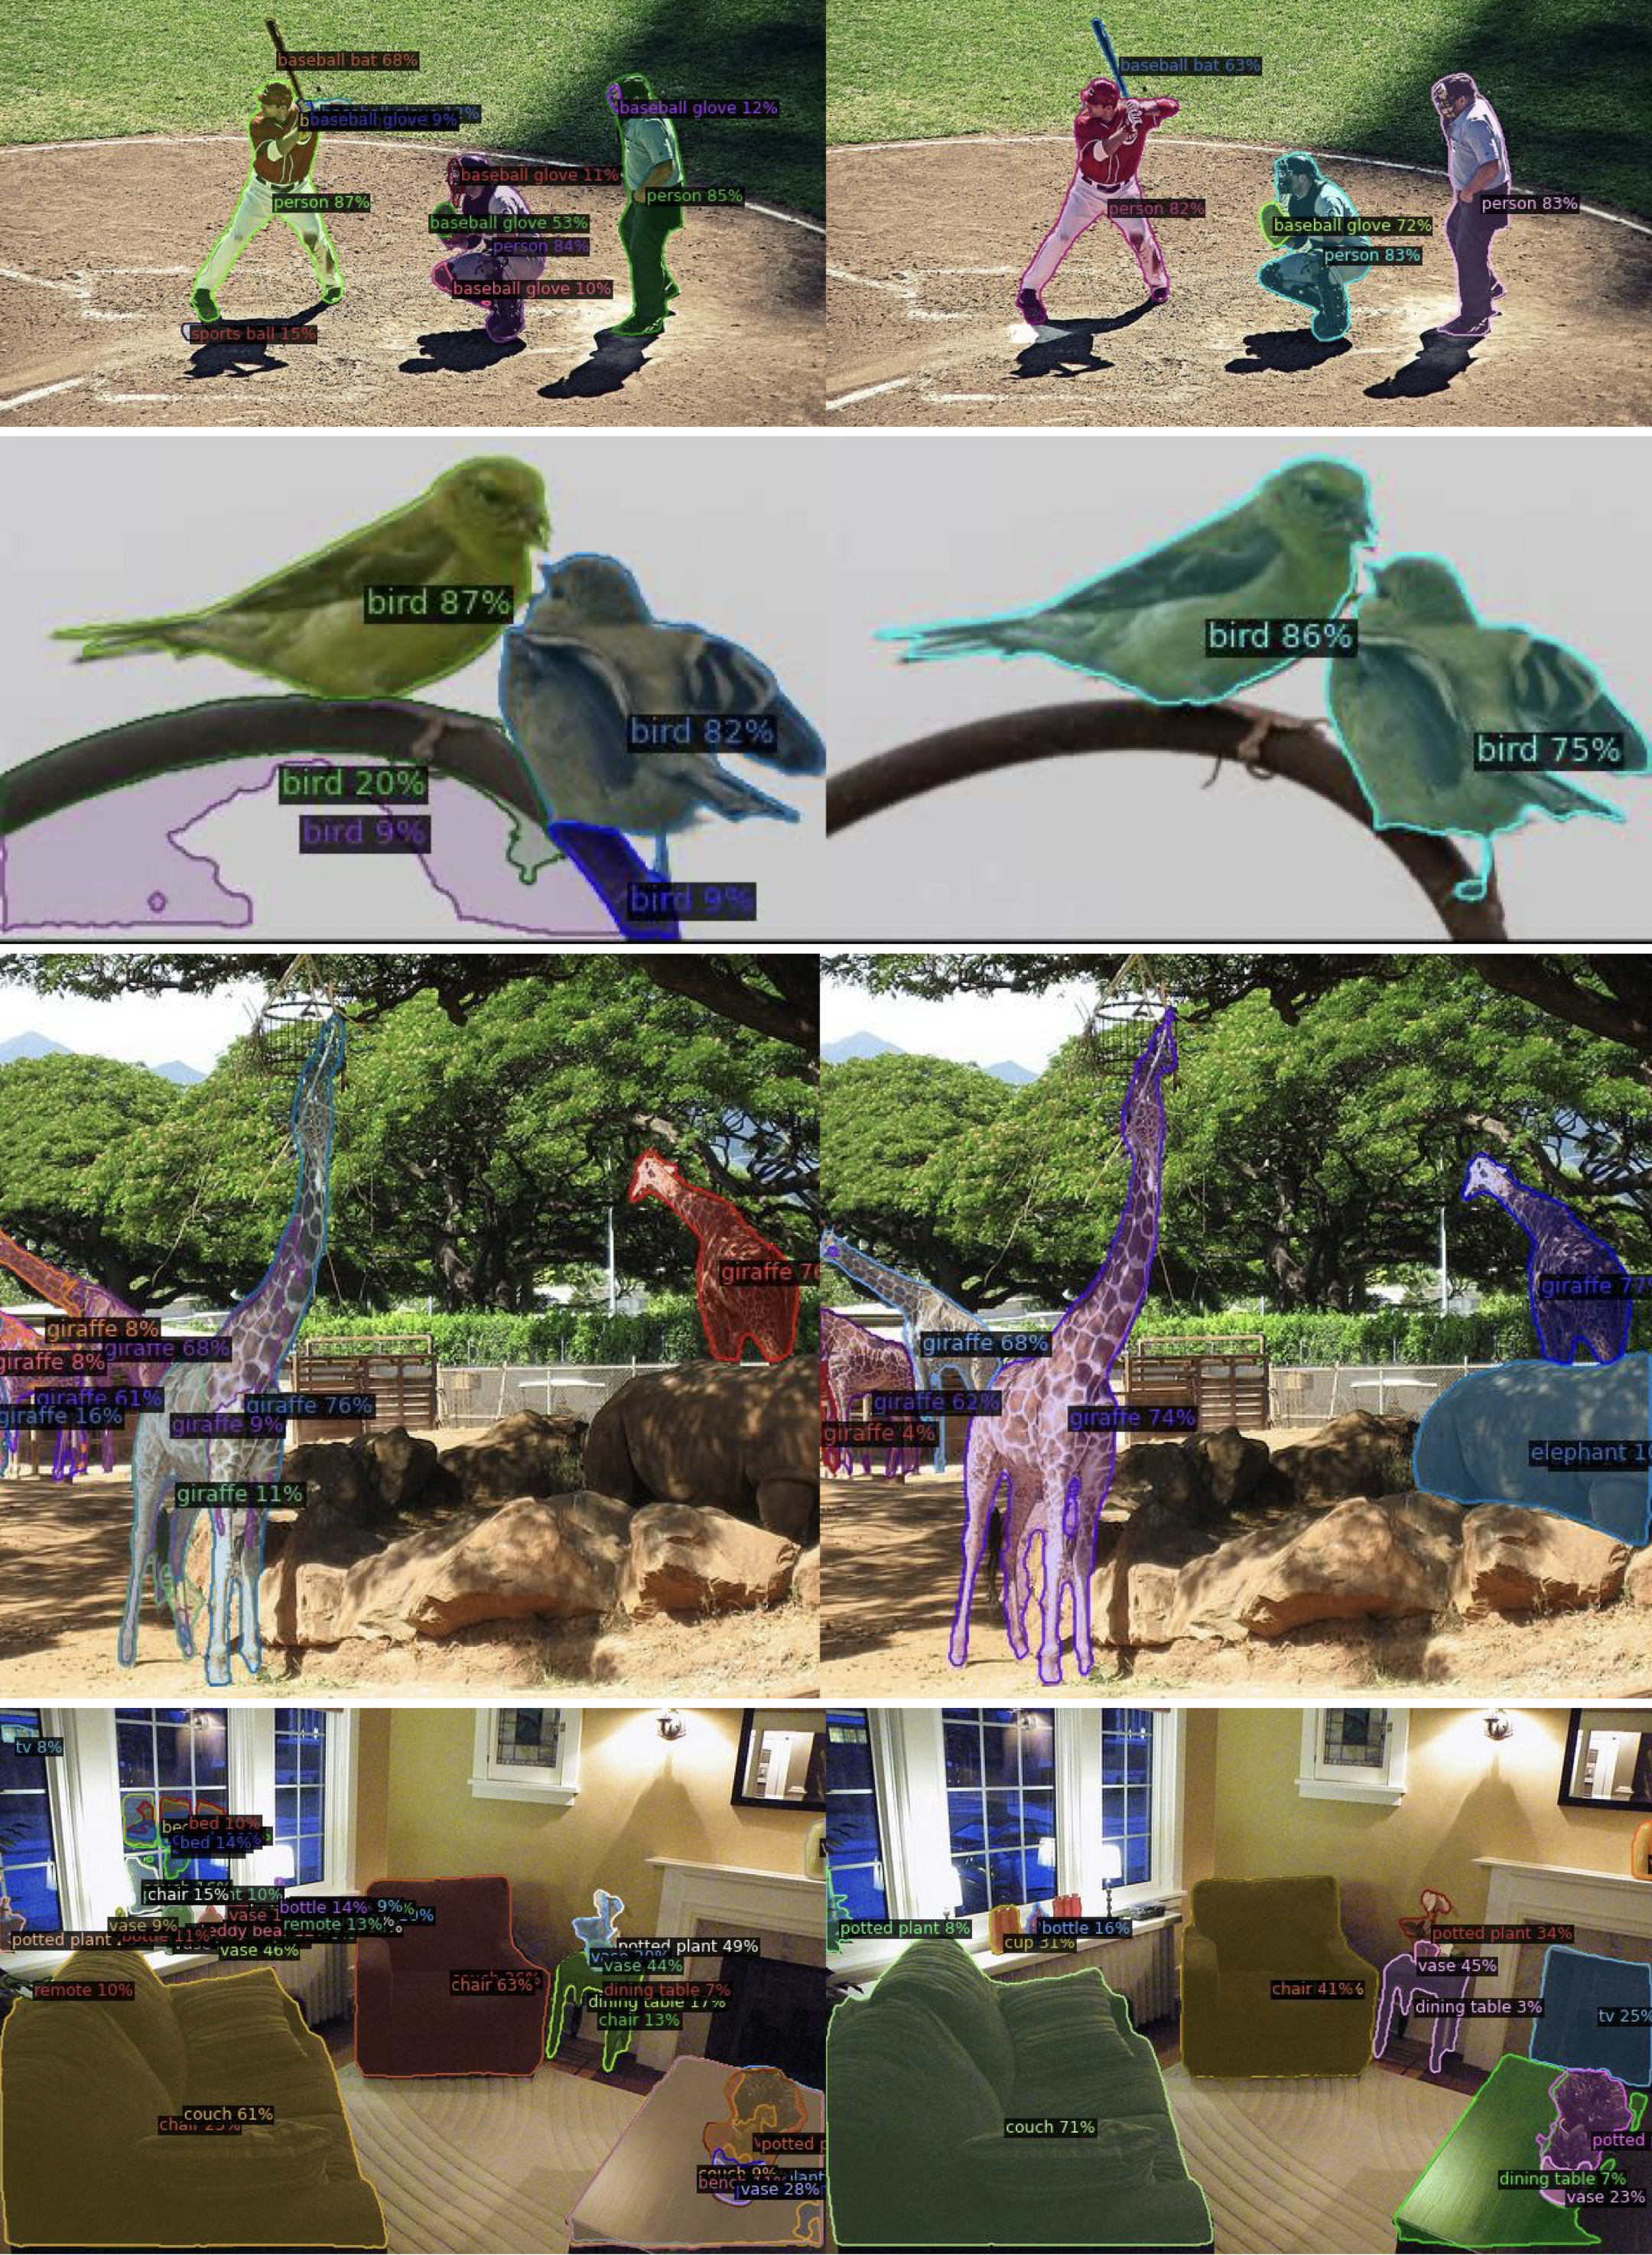}
    \caption{\textbf{Qualitative comparison on COCO-val-2017 dataset}: Images on left are predictions made by SOLOv2, images on right are predictions by our model with Semantic Sorting and Semantic NMS.}
    \label{fig:solovours3}
\end{figure*}
